# Supplementary material for: LagrangianSplats: Divergence-Free Transport of Gaussian Primitives for Fluid Reconstruction
Source: arXiv:2605.09299 source file (2026-05-10)
Supplement: Supplementary file 1 [file supp.tex]

\twocolumn[
% \begin{center}
{\Huge \sffamily
    LagrangianSplats: Divergence-Free Transport of Gaussian Primitives for
Fluid Reconstruction - Supplementary}
        % \vspace{12pt}
		% {\LARGE \newline SUBMISSION ID: 1111}
        \subsection*{
        \hspace{-5pt}
		{\LARGE Ningxiao Tao,} School of Intelligence Science and Technology, Peking University, China  \newline
		{\LARGE Baoquan Chen$^{*}$, } Peking University, China  \newline
		{\LARGE Mengyu Chu$^{*}$, }State Key Laboratory of General Artificial Intelligence, Peking University, China
		}
		%\vspace{-8pt}
% \end{center}
  \vspace{12pt}
]

%\appendix
%\section*{Appendix}
%\label{app:detail}

\noindent
This supplementary document provides additional experimental results and technical details to further support the findings in the main manuscript. The content is organized as follows:

First, we provide more extensive evaluations in diverse and challenging physical environments. Specifically, Sec.~\ref{sec:comp_obstacle} evaluates our method's capability in handling obstacle interactions, while Sec.~\ref{sec:eval_complex} further explores its robustness in highly turbulent scenarios. Finally, Sec.~\ref{sec:details} provides comprehensive implementation details, including network architectures, training strategies, and hyperparameter settings, to facilitate reproducibility.

\begin{table}[bp]
% \centering
\small
\caption{Quantitative comparison on the Sphere dataset, involving complex interactions with a solid obstacle. We benchmark our method against PINF and PICT, both of which employ specialized boundary handling mechanisms. We achieve the highest transport consistency (PSNR, SSIM, LPIPS) and the best physical validity (Div, MSE-$v$, Cos-$v$), demonstrating the superior robustness of our Lagrangian framework in handling boundary conditions.}
\label{tbl:sphereturb_bench}
% 设置列格式：1列左对齐(方法名)，5列居中(数据)
\begin{tabular}{lcccccc}
\toprule
\multirow{2}{*}{Method} & \multicolumn{6}{c}{SphereTurb} \\
\cmidrule(lr){2-7} 
 & PSNR$\uparrow$ & SSIM$\uparrow$ & LPIPS$\downarrow$ & Div$\downarrow$ & MSE-$v$$\downarrow$ & Cos-$v$$\uparrow$ \\
\midrule
PINF & 31.28 & 0.9375 & 0.2090 & 0.002540 & 0.2812 & 0.1646 \\
PICT & 30.23 & 0.9325 & 0.2261 & 0.005083 & 0.8618 & 0.1527 \\
\textbf{Ours} & \textbf{41.00} & \textbf{0.9689} & \textbf{0.1769} & \textbf{0.000061} & \textbf{0.1035}  & \textbf{0.2271}\\
\bottomrule
\end{tabular}
\vfill

\begin{minipage}{\linewidth}
\vspace{4pt}
\raggedright
\rule{48pt}{0.4pt}\par
\small * corresponding authors.
\end{minipage}
\end{table}

\begin{figure}[bp]
    \vspace{-1em}
    \centering
        \begin{minipage}[t]{0.95\linewidth}
            \centering
            \includegraphics[width=\textwidth]{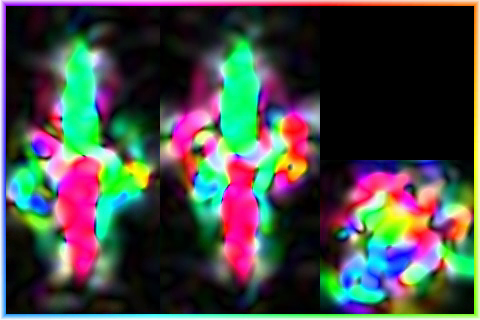}
            \vspace{-20pt}
            \caption*{{Ours}}
            
            \includegraphics[width=\textwidth]{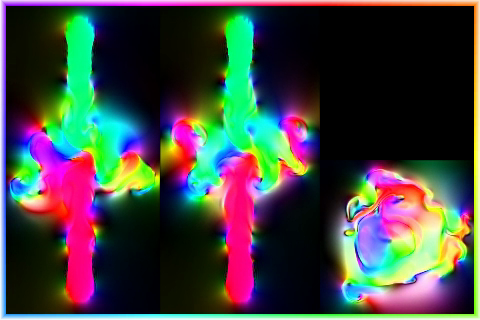}
            \vspace{-20pt}
            \caption*{{Ground Truth}}
        \end{minipage}
    \vspace{-6pt}
    \caption{Velocity field visualization on the Biplume dataset. As observed, our predicted velocity field not only aligns globally with the Ground Truth but also accurately captures fine-grained turbulent details. Quantitatively, our strictly divergence-free construction yields a negligible numerical divergence of $\mathbf{0.000042}$, while achieving a low Velocity MSE of $\mathbf{0.3772}$ and a relatively high Cosine Similarity of $\mathbf{0.1822}$, confirming the high physical accuracy of our reconstruction.}
    \label{fig:velcmpBiplume}
\end{figure}

\vspace{.5em}

\section{Evaluation on Obstacle Interaction}
\label{sec:comp_obstacle}

We evaluate our method on the Sphere dataset to demonstrate its capability in handling solid boundary interactions. Our Lagrangian framework naturally accommodates static obstacles without requiring explicit boundary loss terms. Specifically, within our advection model, static regions are intrinsically represented by Gaussians with zero velocity, ensuring they remain fixed over time. This formulation allows the framework to automatically identify and preserve boundary structures consistent with the observed video. To validate this capability, we explicitly compare our approach against PINF and PICT, both of which incorporate specialized mechanisms for obstacle handling. Quantitative metrics are reported in Table~\ref{tbl:sphereturb_bench}, and qualitative visualizations are presented in Fig.~\ref{fig:velcmpSphere} and Fig.~\ref{fig:resimSphere}.

Regarding the velocity field, as show in Fig.~\ref{fig:velcmpSphere}, visual inspection confirms that our reconstructed velocity correctly vanishes inside the obstacle region and exhibits natural flow separation around the sphere. Quantitatively, our method achieves the lowest Velocity MSE and Divergence, as well as the highest Cosine Similarity, surpassing baselines that employ explicit boundary constraints.

Regarding smoke transport, our method maintains the highest fidelity in the re-simulation task, achieving superior PSNR, SSIM, and LPIPS scores. As illustrated in Fig.~\ref{fig:resimSphere}, our approach produces physically plausible flows that accurately transport smoke around the sphere, preserving intricate details better than previous methods.

These results demonstrate that our framework inherently captures boundary conditions. By leveraging Lagrangian consistency, it achieves higher reconstruction accuracy and physical plausibility compared to prior approaches that rely on manual boundary specifications.

\begin{figure*}[htbp]
    \centering
    
    % ==================================================
    % 第一行设置 (ScalarSyn)
    % ==================================================
    \setlength{\imagewidth}{0.25\textwidth}
    
    % 【关键点1】定义第一行的统一高度。
    % 这里设为 140pt，足以容纳最高的 "Ours" 烟雾。
    % 即使 PINF 很矮，也用这个高度，这样文字才会对齐。
    \def\synHeight{135pt} 
    
    \newcommand{\formattedgraphics}[3]{%
        \begin{tikzpicture}[spy using outlines={rectangle, magnification=2, connect spies}]
          % 1. 先画一个黑底，防止图片不够高时顶部出现白边 (可选)
          \fill[black] (0, 5pt) rectangle (\imagewidth, \synHeight);
          
          % 2. 统一裁剪高度
          \clip (0, 5pt) rectangle (\imagewidth, \synHeight);
          
          % 3. 插入图片
          \node[anchor=south west, inner sep=0] at (0,0){\includegraphics[width=\imagewidth]{#1}};
          
          % 4. 文字位置：基于 \synHeight 进行相对定位，保证所有文字距离顶部的距离一致
          % 方法名：位于顶部向下约 12pt 的位置
          \node[anchor=north west,text=white] at (.02\imagewidth, \synHeight - 5pt){\sffamily\footnotesize\textbf{#2}};
          
          % PSNR值：位于方法名下方
          \node[anchor=north west,text=white] at (.02\imagewidth, \synHeight - 15pt){\sffamily\scriptsize #3};
        \end{tikzpicture}%
    }

    % \formattedgraphics{fig/sphereturb_resim/PINF_044.png}{PINF}{PSNR 31.28}%
    \formattedgraphics{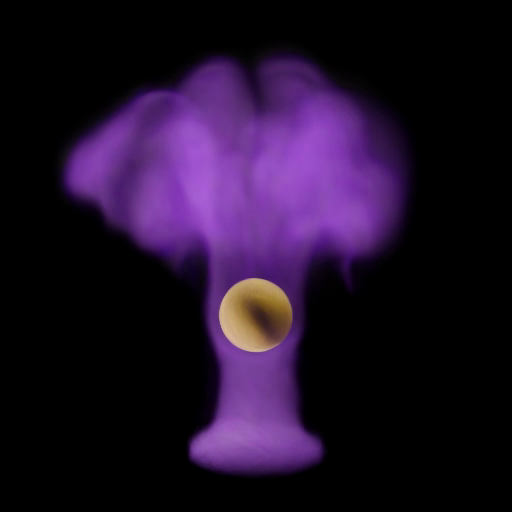}{PINF}{}%
    \hspace{-0.18cm}%
    % \formattedgraphics{fig/sphereturb_resim/PICT_044.png}{PICT}{PSNR 30.23}%
    \formattedgraphics{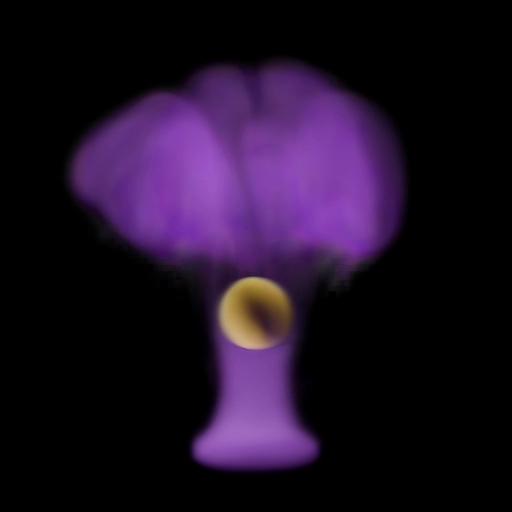}{PICT}{}%
    \hspace{-0.18cm}%
    % \formattedgraphics{fig/sphereturb_resim/DFKGS_044.png}{Ours}{PSNR \textbf{41.00}}%
    \formattedgraphics{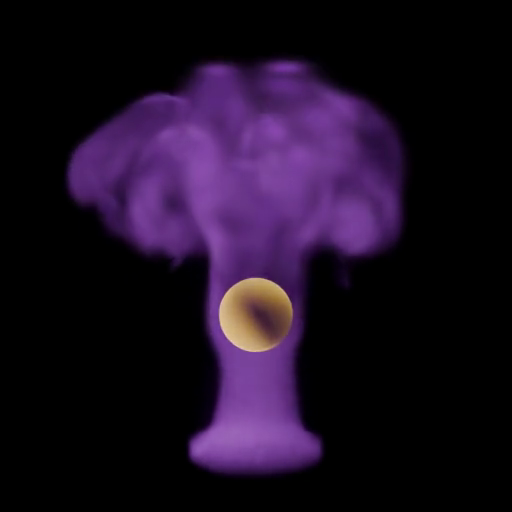}{Ours}{}%
    \hspace{-0.18cm}%
    \formattedgraphics{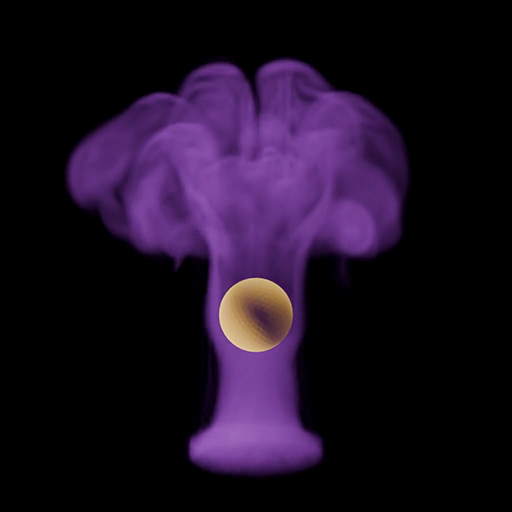}{Ground Truth}{}%
    \\
    \vspace{-6pt}
    \caption{Comparison of re-simulation results on the Sphere scene. \rv{We visualize a late-time snapshot of the smoke density advected by the reconstructed velocity fields of different methods.} Baseline approaches (PINF, PICT) fail to maintain the smoke's structural integrity over time, leading to noticeable dissipation or inaccurate transport around the obstacle. Our method, conversely, produces a physically plausible flow that smoothly transports smoke around the sphere, preserving sharp details and achieving the highest visual fidelity compared to the Ground Truth.}
    \label{fig:resimSphere}
\end{figure*}

% \begin{figure*}[htbp]
%     \centering
%     \begin{minipage}[t]{\linewidth}
%         \centering
%         \begin{minipage}[t]{0.32\linewidth}
%             %\centering
%             \includegraphics[width=\linewidth]{fig/sphereturb/PINF_018.png}
%             \vspace{-20pt}
%             \caption*{{PINF}}
%             \includegraphics[width=\linewidth]{fig/sphereturb/PICT_018.png}
%             \vspace{-20pt}
%             \caption*{{PICT}}

%         \end{minipage}%
%         % \hfill
%         % \\
%         \begin{minipage}[t]{0.32\linewidth}
%             \centering
%             \includegraphics[width=\textwidth]{fig/sphereturb/DFKGS_018.png}
%             \vspace{-20pt}
%             \caption*{{Ours}}
            
%             \includegraphics[width=\textwidth]{fig/sphereturb/gt_018.png}
%             \vspace{-20pt}
%             \caption*{{Ground Truth}}
%         \end{minipage}
%     \end{minipage}
%     \vspace{-6pt}
%     \caption{Visualization of reconstructed velocity fields on the Sphere scene. As observed, PINF and PICT struggle to fully resolve the flow around the obstacle, exhibiting either blurry boundaries or artifacts. In contrast, our method correctly identifies the static obstacle region, where the velocity naturally vanishes, and reconstructs a clean flow field with clear separation around the sphere. This visual evidence aligns with our quantitative results, confirming that our framework inherently respects boundary conditions.}
%     \label{fig:velcmpSphere}
% \end{figure*}
\begin{figure}[bp]
    \centering
    
    % 第一行
    \begin{minipage}[t]{0.48\linewidth}
        \centering
        \includegraphics[width=\linewidth]{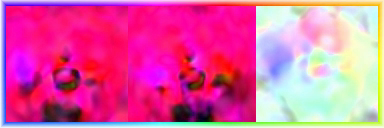}
        \vspace{-20pt}
        \caption*{{PINF}}
    \end{minipage}
    \begin{minipage}[t]{0.48\linewidth}
        \centering
        \includegraphics[width=\linewidth]{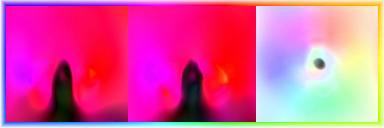}
        \vspace{-20pt}
        \caption*{{PICT}}
    \end{minipage}
    
    % \vspace{10pt} % 第一行和第二行之间的垂直间距
    
    % 第二行
    \begin{minipage}[t]{0.48\linewidth}
        \centering
        \includegraphics[width=\linewidth]{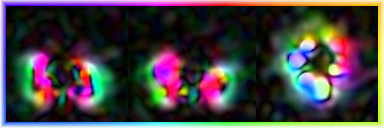}
        \vspace{-20pt}
        \caption*{{Ours}}
    \end{minipage}
    \begin{minipage}[t]{0.48\linewidth}
        \centering
        \includegraphics[width=\linewidth]{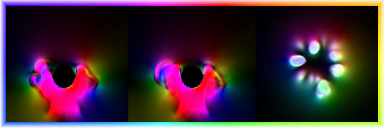}
        \vspace{-20pt}
        \caption*{{Ground Truth}}
    \end{minipage}
    
    \vspace{-6pt}
    \caption{Visualization of reconstructed velocity fields on the Sphere scene. As observed, PINF and PICT struggle to fully resolve the flow around the obstacle, exhibiting either blurry boundaries or artifacts. In contrast, our method correctly identifies the static obstacle region, where the velocity naturally vanishes, and reconstructs a clean flow field with clear separation around the sphere. This visual evidence aligns with our quantitative results, confirming that our framework inherently respects boundary conditions.}
    \label{fig:velcmpSphere}
\end{figure}

\begin{table*}[htbp]
    \centering
    \caption{Detailed dataset statistics, including frame counts, hyperparameter configurations, and training costs for all experimental scenes. Benefiting from the rapid rasterization of 3DGS and the efficient evaluation of DFKs, our framework achieves high-fidelity reconstruction with remarkably low computational overhead. As shown, the total training time typically ranges from 30 minutes to 3 hours on a single RTX 4090 GPU, demonstrating the practicality of our approach for handling high-resolution 4D fluid dynamics on consumer-level hardware.}
    \label{tbl:hyperparameters}
    \small % 适当缩小字体以适应页面宽度
    \setlength{\tabcolsep}{6pt} % 如果列增加了，可能需要稍微调小一点间距，建议 6pt 或 5pt
    \begin{tabular}{l c c ccc ccc}
        \toprule
        \multirow{2}{*}{\textbf{Scene}} & \multirow{2}{*}{\textbf{Frames}} & \multirow{2}{*}{\textbf{Window Size $w$}} & \multicolumn{3}{c}{\textbf{Loss Weights}} & \multicolumn{2}{c}{\textbf{Iterations}} & \multirow{2}{*}{\textbf{Training Time (min)}} \\
        \cmidrule(lr){4-6} \cmidrule(lr){7-8} % 注意这里 cmidrule 的范围因为加了一列顺延了
         & & & $\lambda_{\text{aniso}}$ & $\lambda_{\text{reg}}$ & $\lambda_{\text{vor}}$ & Warm-up & Sliding & \\
        \midrule
        ScalarSyn (Sec.~\ref{sec:comp_standard})  & 30 & 10 & 10.0 & 0.01 & 0.1 & 500 & 100 & 28 \\
        ScalarReal (Sec.~\ref{sec:comp_standard}) & 120 & 10 & 10.0 & 0.01 & 0.1 & 500 & 100 & 170 \\
        Sphere (Sec.~\ref{sec:comp_obstacle})    & 45 & 10 & 10.0 & 0.005 & 0.1 & 500 & 100 & 49 \\
        Biplume (Sec.~\ref{sec:eval_complex})     & 30 & 5  & 10.0 & 0.005 & 0.1 & 600 & 200 & 56 \\
        \bottomrule
    \end{tabular}
\end{table*}

\section{Evaluation on Complex Dynamics}
\label{sec:eval_complex}

% \begin{table}[htbp]
% \centering
% \small
% \begin{tabular}{lccccc}
% \toprule
% \multirow{2}{*}{Method} & \multicolumn{5}{c}{Biplume} \\
% \cmidrule(lr){2-6} 
%  & PSNR$\uparrow$ & SSIM$\uparrow$ & LPIPS$\downarrow$ & Div$\downarrow$ & MSE-$v$$\downarrow$ \\
% \midrule
% \textbf{Ours} & 37.70 & 0.9764 & 0.07577 & 0.000042 & 0.3772 \\
% \bottomrule
% \end{tabular}
% \vspace{1em}
% \caption{Quantitative results on the Biplume scene.}
% \label{tbl:biplume_bench}
% \end{table}

To further investigate the robustness of our method in highly chaotic scenarios, we evaluate it on the Biplume dataset, which features intense turbulence and rapid motion. Quantitative metrics and qualitative visualizations are presented in Fig.~\ref{fig:teaser} and Fig.~\ref{fig:velcmpBiplume}. Despite the complexity of the flow, our method demonstrates robust capability in capturing intricate turbulent details. The reconstructed velocity field successfully drives the smoke evolution with high fidelity, while maintaining strict physical incompressibility throughout the volume. These results confirm the applicability of our framework to complex fluid dynamics.

\section{Implementation Details}
\label{sec:details}

We implement our framework using PyTorch, utilizing the Adam optimizer for all parameters. For the 3D Gaussian Splatting optimization, we follow the standard learning rate schedule~\cite{kerbl2023gaussian_splatting}. For the velocity field parameterized by DFK, we initialize the learning rate at $0.1$ and apply an exponential decay scheduler, reducing it to $0.001$ by the end of training. Detailed dataset statistics, including frame counts, hyperparameter configurations, and training costs for all experimental scenes can be found in Table~\ref{tbl:hyperparameters}. All experiments are conducted on a single NVIDIA RTX 4090 GPU.

Regarding computational efficiency, our method leverages the fast rasterization of 3D Gaussian Splatting combined with the kernel evaluation of the DFK representation. Consequently, the total training time typically ranges from 30 minutes to 3 hours, depending on scene complexity. This efficiency makes our framework practical for reconstructing high-resolution 4D fluid dynamics on consumer-level hardware.
